# Supplementary material for: In situ compensation method for high-precision and high-sensitivity integral magnetometry
Source: arXiv:1809.02346 ancillary file (2019-07-05)
Supplement: Supplementary file 1 [file S.Info_v4.0.pdf]

# Supplementary Information to:

# *In situ* compensation method for high-precision and high-sensitivity integral magnetometry

K. Gas[1, *] and M. Sawicki[1, †]
[1] *Institute of Physics, Polish Academy of Sciences, PL-02668 Warsaw, Poland*

## CONTENTS

S1. Equipment related nonlinearities in SQUID magnetometers 1
S2. Experimental benefits of *in situ* compensation 2
S3. Determination of $\mu_G$ 3
S4. The role of the $\gamma$ factors 4
S5. Setting of the measurements 5

References 6

## S1. Equipment related nonlinearities in SQUID magnetometers

The scale of the typical output instabilities of a rather well maintained MPMS systems is exemplified in Fig. S1, where we present some $m(H)$ measurements of a test piece of a sapphire substrate. These $m(H)$ have been collected over a period of nearly two years using, in general, the same experimental sequence and identical in design and construction sample holders made from 1.5 mm wide and about 20 cm long Si strips. An example of such a "classical" design sample holder is depicted in the Fig. 3 (a) of the main part. The bare magnetic response of the sapphire is "negative" (diamagnetic) and quite linear in $H$, so to visualize both the deviations from the ideal diamagnetic response and the SQUID output instabilities, all $m(H)$ are compensated by a linear $\alpha_L H_{\mathrm{set}}$ term:

$$m_{\mathrm{comp}}(H_{\mathrm{set}}) = m(H_{\mathrm{set}}) - \alpha_L H_{\mathrm{set}}, \tag{S1}$$

where for the presented here about $5 \times 5 \times 0.33$ mm$^3$ sample a value of $\alpha_L = -1.31 \times 10^{-8}$ emu/Oe is adopted, and $H_{\mathrm{set}}$ are the magnetic field amplitudes reported in the *.dat output files produced by MultiVu (the MPMS measurement software). Concerning the magnitude of the numerical compensation, the full scale in panel (a) of 2 $\mu$emu corresponds to about 99% and 99.8% compensation at 20 and 70 kOe, respectively. In panel (b) the full scale of 15 $\mu$emu corresponds to 98% of compensation. Both cases represent the minimum compensation levels required in the determination of Mn contents or the magnetic anisotropy at high fields for thin or dilute magnetic films.

The first feature that sticks out from the top panels of Fig. S1 is a sizable curvature of all $m_{\mathrm{comp}}(H)$. Its existence, either intrinsic to this sapphire sample - due to residual contamination or other structural defects, or extrinsic - caused by the non-ideal $H_{\mathrm{set}} \leftrightarrow H_{\mathrm{real}}$ correspondence in the magnetometer, is not a particularly worrying feature, at least as long as it does not change between nominally equivalent measurements. Remaining the same for the relevant consecutive measurements it would be eradicated easily by the subtraction approach to the sensitive magnetometry.

The truly troublesome features of the results presented in Fig. S1 are: (i) the substantially varying in time magnitude of $m_{\mathrm{comp}}(H)$, (ii) the presence of sudden "jumps" or "kinks" occurring randomly at different magnetic fields [the most prominent are indicated by the arrows in panel (a)], and (iii) a lack of a symmetry of the magnitude of $m_{\mathrm{comp}}(H)$ for positive and negative fields, expected at least at 300 K. Concerning the first point, it can be noted that the variation in magnitude of $m_{\mathrm{comp}}(H)$ at $\sim 70$ kOe remained less than $\sim 2$ $\mu$emu in a "short" time scale of about a year time (measurements A-F), but it has been found increased to $\sim 10$ $\mu$emu after another year time (measurement G). This finding very strongly points to the fact that in the traditional approach to precision magnetometry no one can rely on a "universal background curve" established once for all of the samples grown on the same type of substrates and investigated in months or years lasting project. It has to be underlined, that the tested sample, the initial prime reference in the study, has been kept in a pristine condition – frequently cleaned in organic solvent as well and in HCl. The authors have not established what was the underlying reason of such a wrongdoing of the system. The long term experience with MPMS systems indicates that some tear and wear of the RSO transport mechanism seems to be most likely.

On the other hand, the results presented in Fig. S1 clearly illustrate the reason why in the precision magnetometry the signal of the substrate cannot be simply approximated by a linear in $H$ dependency (without an independent check that it really is).

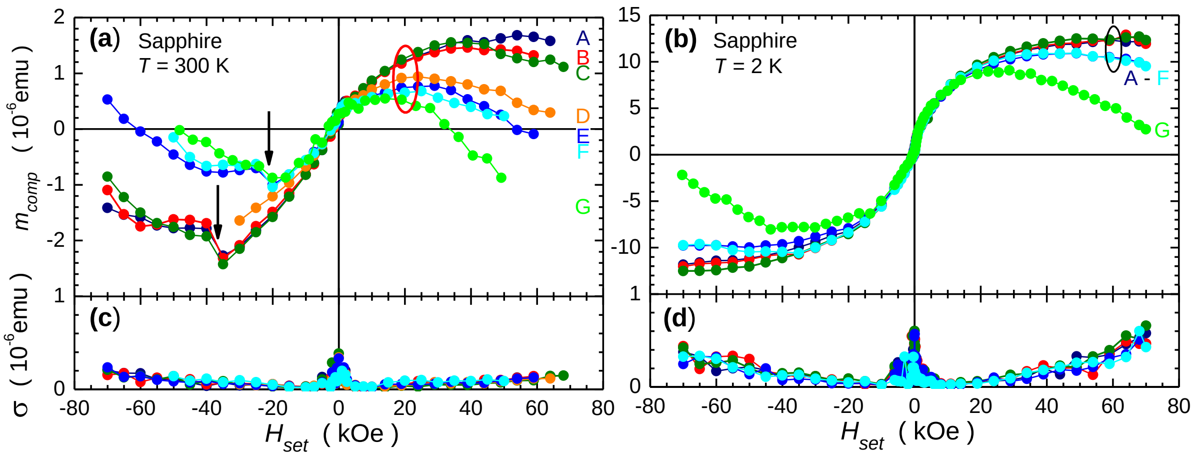


FIG. S1. Magnetic field $H_{\rm set}$ dependence of a nonlinear part of the magnetic moment $m_{\rm comp}$ of a sapphire sample recorded at (a) 300 and (b) 2 K in a short time frame (one month, curves A - E), a year later (curve F) and again after a year (curve G). All the experimental recorded magnitudes of the magnetic moment of the sample are linearly compensated in $H_{\rm set}$ by the same coefficient $\alpha_L = -1.31 \times 10^{-8}$ emu/Oe [Eq. (S1)]. $H_{\rm set}$ are the magnitudes of magnetic field recorded in the MPMS magnetometers *.dat output files. All these curves have been obtained by sweeping the field one way from positive to negative values. The arrows indicate places where sudden shifts of $m_{\rm comp}$ ("jumps") are taking place. The red oval in (a) marks a spread of the magnitudes of magnetic moment recorded in another two years long experiment for an equivalent sample (Fig. 2 in the main text). For the clarity of presentation the corresponding standard deviations $\sigma$ for these points are given in separate panels: (c) for 300 K and (d) for 2 K. The sizable magnitude of $\sigma$ at weak fields results from a strong magnetic flux creep and escape in the superconducting magnet. Effectively, it means that even despite operating the magnet in the persistent mode, during the act of the measurement the field in sample chamber is not stable and fluctuates to some degree, what is sensed by the SQUID pick-up coils and randomly affects the magnitude of each experimental point.

## S2. Experimental benefits of *in situ* compensation

The improvement in experimental quality is exemplified in Fig. S2, where we collect magnetization curves measured with the *in situ* compensation of various sapphire pieces investigated in the course of reported here studies. This is an arbitrary, but a representative choice of the sapphire substrates available on the market, including the same sapphire sample from Fig. 1 of the main part and Fig. S1 (sample C). To set a common frame for all these results, similarly as in Fig. S1, a linear in $H_{\rm set}$ compensation is applied [Eq. (S1)]. Because the samples are physically different, this time various coefficients $\alpha_L$ are needed. They are adjusted independently for each sample to obtain a flat, field independent response at high fields at 300 K, Fig. S2 (a). Then, the same $\alpha_L$ is applied to the corresponding data obtained at 2 K, panel (b). This purely technical approach to the presentation of the results has been adopted here to underline a radically increased consistency of the data. In particular, there are no "jumps", and the results are fairly symmetrical with respect to the origin of the graphs. It is worth further noting that the scales of panels (a), (c) and (d) are five-fold expanded with respect to their counterparts in Fig. S1, meaning in particular that the *in situ* compensation reduces the noise level associated with $V(z)$ reduction to $m$. On the other hand, the sizably reduced overall curvatures of $m_{\rm comp}(H_{\rm set})$ at stronger fields are in fact of a lesser importance - this is actually an expected effect here. Indeed, there would be no net flux measured using a compensational sample holder (CSH) with a matching sample fitted in the gap, so the $m(H)$ should be $H$-independent and $m(H) \equiv 0$, unrespectable if $H_{\rm set} = H_{\rm real}$, or not.

The scale in panel (b) remains the same as in the corresponding panel of Fig. S1, mainly because of a strong, paramagnetic-like, response exerted by pieces A and B. Both this feature and the clear FM-like appearance in weak fields at 300 K underline the important practical issue that the available sapphire substrates differ substantially in the concentration of residual magnetically active centers or contaminants. Even the employed here CSH possesses a residual magnetic signature - we routinely register a weak remnant FM-like moment of about 0.1 – 0.2 $\mu$emu at $T$ = 300 K, seen here for samples A, C, D, and E. This is further corroborated by an observation of an inverted ferromagnetic-like response in sample B, indicative that this sample contains less FM-like contaminants than the central part of the CSH in which the measurement takes place. On the other hand, a single test measurement at room $T$ proves not really sufficient – the same sample B examined further down to 2 K yielded (as well as samples A and C) a very strong, prohibitive for construction purposes, temperature dependent paramagnetic response. In this particular respect, pieces D and E look very consistent in the whole $T$-range, yielding relatively weak in magnitude and weakly temperature dependent magnetic response. In this respect, the data

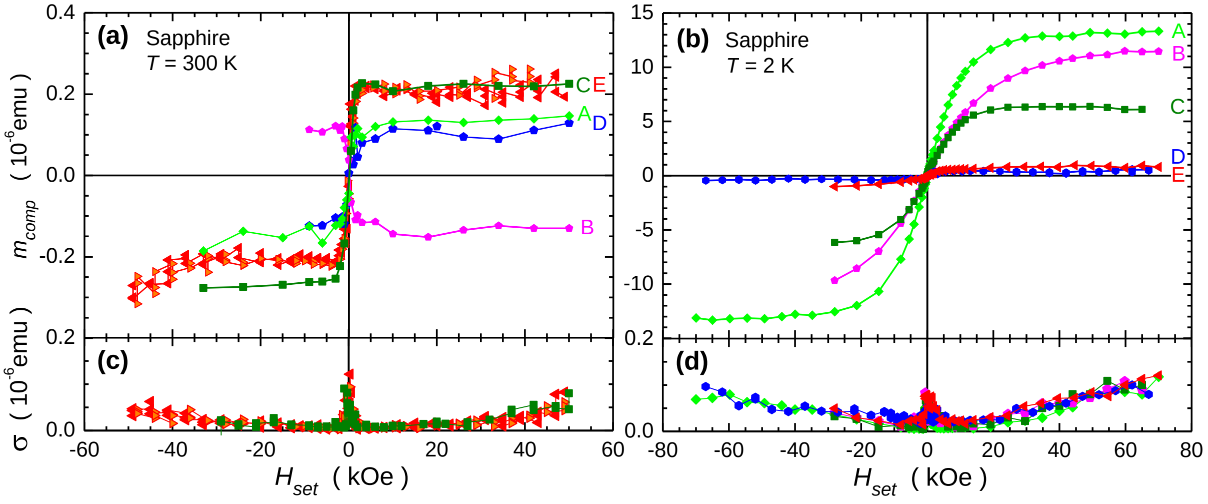


FIG. S2. Magnetic field $H_{\rm set}$ dependence of a nonlinear part of the magnetic moment $m_{\rm comp}$ of a few sapphire test samples (including that presented in Fig. S1 - sample C) measured at (a) 300 and (b) 2 K, with the *in situ* compensation realized in the compensational sample holder [presented in Fig. 3 (c) in the main text]. All the experimentally recorded magnitudes of the magnetic moment are linearly compensated in $H_{\rm set}$ by individually adjusted for each of the sample coefficients $\alpha_L$ [Eq. (S1)] to obtain a flat $H$-response at 300 K. $H_{\rm set}$ are the magnitudes of magnetic field recorded in the MPMS magnetometers *.dat output files. Except for sample E at 300 K, all the curves have been recorded during one way $H$-sweep from positive to negatives values. Left and right pointing triangles indicate data obtained for sample E during sweeping the field down from 50 kOe and up from -50 kOe, respectively.

collected in Fig. S2 underline the importance of a preselection of the most possible pristine substrate materials if sensitive magnetic studies are planned.

## S3. Determination of $\mu_G$

Equations 1 and 2 from the main text state that when both the investigated specimens and the reference sample(s) are so similar that $\beta \simeq 0$, the contribution of the empty CSH to the researched signal of interest $m_{\rm X}$ can be neglected. But this is rather unlikely case in a long run so the full Eq. 2 has to be used on a daily basis. For this the magnitude of $\mu_G\gamma_{\rm G}$, that is the product of the mass of the missing material between the compensating strips and its size correcting factor has to be established.

To this end we take advantage of the test $m(H)$ measurements performed in the all-sapphire CSH with about 5.2 mm gap between the sapphire compensating strips for differing in size and weight sapphire specimens (they are of a different origin too). Some of the corresponding $m_{\rm comp}(H)$ dependencies are presented in Fig. S2 (a). Since at room temperature $m_{\rm comp}(H)$ at $H \gtrsim 0.5$ T linearly depends on $H$ in nearly all cases, a plot of $\alpha_L$ [the coefficient required to flat out the experimental $m(H)$, see Eq. S1] as the function of the product of mass times $\gamma$ of these specimens yields the magnitude of $\mu_G\gamma_{\rm G}$ at the $x$-intercept of this dependency. The procedure is exemplified in the main panel of Fig. S3. The best assessment is obtained from the points representing specimens of very similar shapes and weights to that of the gap ($\simeq 5 \times 5$ mm$^2$ in this case), since they group very close to the sought $x$-intercept. However, it is worth noting that the magnitudes of $\alpha_L$ of samples which $\mu\gamma$ differ considerably from that of the gap also fall on the same (linear) trend established by the point representing the empty CSH ($\mu = 0$) and the rest of the points.

There are generally three groups of points. These of $\alpha_L \cong 0$ correspond to $5 \times 5$ mm$^2$ samples of the same thickness as the compensating strips, so their $\mu\gamma$ are very close to $\mu_G\gamma_{\rm G}$ and for them the compensation degree approaches 100%. The second group of points with $\alpha_L \cong -0.0033$ $\mu$emu/Oe corresponds also to $5 \times 5$ mm$^2$ sapphire bits but of greater masses, since they are thicker, about 0.4 mm. The third group with $\alpha_L \simeq 0.0025$ $\mu$emu/Oe corresponds to $\simeq 5 \times 4$ mm$^2$ rectangular samples. The two triangles in this group mark results obtained for one of such samples which has been mounted in this about $5 \times 5$ mm$^2$ CSH either with its longer side oriented along the length of CSH (the right-pointing triangle) or perpendicularly (the top-pointing one). This is exemplified in Fig. S4. The observed magnitudes of $\alpha_L$ differ in both these cases, but they fall on the the same linear dependency established by the other points when proper magnitudes of $\gamma$ are applied for these two configurations. We expand on the role of $\gamma$ and its proper assignment with regard to the sample's orientation in the next section of this Supplementary Information.

It has to be added that in principle instead of $\alpha_L$ one can take results of single measurements performed at one, sufficiently strong magnetic field $H_S$, say between 20 and 50 kOe. However, such a simplification will yield

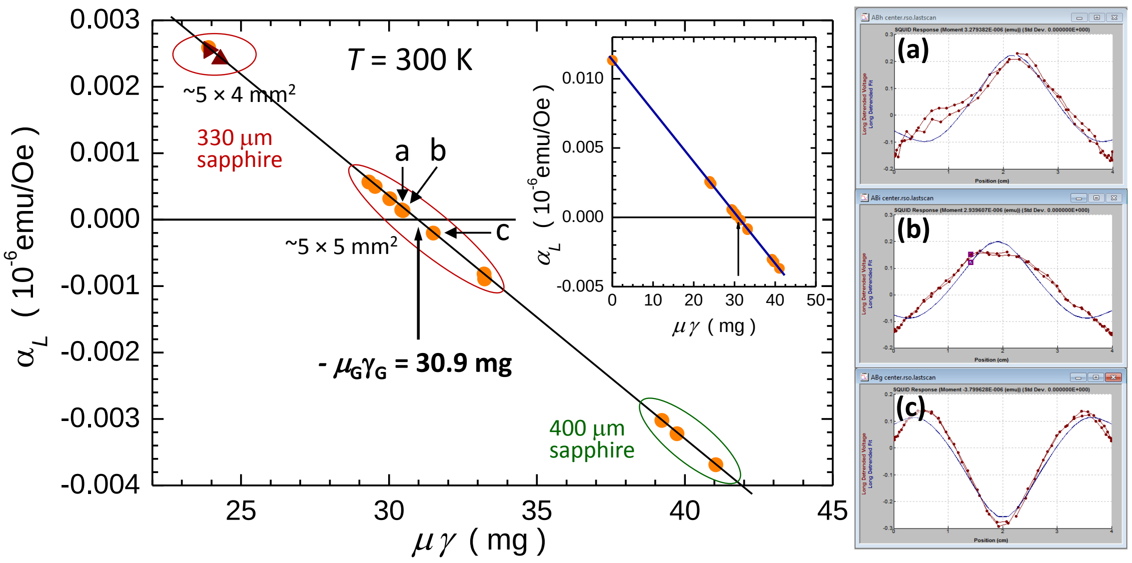


FIG. S3. (Main panel) Illustration of the experimental method of establishing $\mu_G\gamma_G$ (the product of the mass of the missing material between the compensating strips and of the "geometrical factor" corresponding to this gap) - case of the the all-sapphire compensational sample holder (CSH) assembly depicted in Fig. 4 (c) in the main text. The searched magnitude of $\mu_G\gamma_G = -30.9$ mg is indicated by the arrow. The sign "–" reflects an opposite magnetic response of the gap between the compensating strips and a negative value should enter Eq. 2 (main text) in a case of diamagnetic compensation. Bullets represent magnitudes of coefficients $\alpha_L$ describing the slope of the linear (high field) part of the room temperature $m(H)$ for tested sapphire samples. The two triangles depict $\alpha_L$ and $\mu\gamma$ for the same rectangular $\simeq 5 \times 4$ mm$^2$ sapphire sample mounted in the CSH either along the longer edge (right pointing triangle) or along the shorter one (top pointing one) - this is depicted in Fig. S4. Panels (a - c) depict the shapes of the centering scans obtained using the reciprocating sample option mode of measurement in the already pre-centered CSH (the centering issue is discussed in section S5 of this Supplementary Information) with three samples of close matching $\mu\gamma$ to that of the compensating gap. The "Long Detrended Voltage" (brown bullets and lines) is the direct representation of $V(z)$ with a compensation for system drifts applied. Its amplitude corresponds to the strength of the measured moment. Dark blue lines indicate point dipole ideal response function $\Upsilon(z)$ fitted using the linear regression mode. The established for these particular samples coefficients $\alpha_L$ are indicated by the arrows in the main panel.

a correct magnitude $\mu_G\gamma_G$ only when $m(H_S)/m(H_w) \cong H_S/H_w$, where the weak field magnitude $H_w$ ranges between $\sim 1$ to 5 kOe, i.e. when the magnetic response of the sample is fairly proportional to $H$.

We summarize here that when all the described above precaution are taken into account only 2–3 experimental values of $\alpha_L$ plus that of the empty gap are practically sufficient to accurately establish $\mu_G\gamma_G$.

## S4. The role of the $\gamma$ factors

The problem of non-zero specimen dimensions and their influence on the strength of the coupling with pick-up coils [this affects both amplitude and the shape of the $V(z)$] has been recognized already very early[1–3] and the reader can find plenty of correction factors for various experimental configurations in these papers. Correction factors cannot be omitted in the precision magnetometry conducted on typical macroscopically large samples if such is based on the MultiVu software, since the magnitude of the measured moment is established in the point object approximation, and only in this case the size correcting factor $\gamma = 1$. The typical specimens of layered material assume areas of 20 - 30 mm$^2$, so a post-measurement correction is needed to give the account for the sample's extent along the $z$ axis (that is along the sample holder) and perpendicularly to it (radially). Magnitudes of $\gamma$ for most frequently met cuboidal shapes are listed in Table 1 of ref. 4, for the other intermediate lengths the correct values of $\gamma$ can be obtained from a linear interpolation of the data in this table or from ref. 3. For example for a $5 \times 5$ mm$^2$ square sample $\gamma \cong 0.97$ in parallel orientation[3,4], so the necessary correction amounts to $+3\%$ and omitting it will practically invalidate the outcome of Eq. 2 from the main text.

Additional caution has to be exerted when it comes to investigation of irregularly shaped samples. It is because the magnitude of $\gamma$ depends not only on the shape itself but also on how this shape is oriented with respect to the axis of the gradiometer $z$.[3,4] As the rule of the thumb $\gamma$ is smaller when the sample is mounted with its longer side oriented along $z$ and greater when perpendicularly to it.

This effect gets sizably magnified in a CSH. As an example we consider the case of the rectangular sample whose established magnitudes of $\alpha_L$ are marked by the

triangles in Fig. S3. The corresponding specific experimental configurations are illustrated in Fig. S4. It becomes immediately evident that placing this $4 \times 5$ mm$^2$ rectangular piece in the square $5 \times 5$ mm$^2$ gap in its two basic orientation: (L) with the longer side parallel to $z$, and (s) perpendicular to it, generates two completely different pairs of elongated voids (marked by hatched boxes) in the otherwise uniform and very long object. In the integral magnetometry the latter does not exert any flux. The magnetometer senses only an opposite flux exerted by these two pairs of voids. However, despite the fact that both pairs of voids have the same volume and that they correspond to the same material, the flux they exerts couples completely differently to the magnetometer. The two voids in the first case, Fig. S4 (L), are exclusively located at the edges of the sample holder, that is at the farthest possible distance from $z$, so their fluxes couple stronger with the pick-up coils than the flux exerted in configuration (s), in which majority of the flux originates from the locations which are much closer to $z$, i.e. where the coupling is weaker, cf. Fig. 2 b in ref. 4. Now, it has to be observed that even without the compensating strips the difference in $\gamma$ for these two configuration (about 1.7% for such a shape) results in the same difference in reported magnitudes of $m$. However, with the strips applied, the qualitatively different location of the voids in both cases increases the difference in the response to about 5.5%, i.e. it gets three times larger. In absolute numbers, an improper assignment or omission of $\gamma$ may lead to an absolute error in $m_{\mathrm{x}}$ as large as 10 $\mu$emu at 50 kOe, i.e. exceeding by far the requirements for the precision magnetometry.

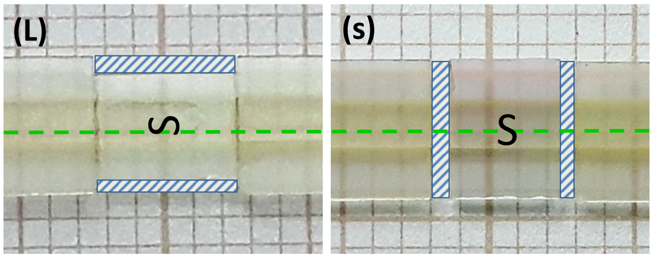


FIG. S4. The two experimental configurations in which the rectangular $5 \times 4$ mm$^2$ sapphire sample $\boldsymbol{S}$ has been mounted in the $5 \times 5$ mm$^2$ gap of the all-sapphire compensational sample holder for the determination of the "mass" of the gap, as detailed in Fig. S3. Each of the configurations results in differently located with respect to the magnetometer axis (green dashed line) pairs of voids in sapphire, marked here by blue hatched boxes. They are the only effective sources of the magnetic flux, but despite of the equal volume they couple differently to the magnetometer pick-up coils. This may lead to differences as large as $10^{-5}$ emu at $H > 50$ kOe.

## S5. Setting of the measurements

We start from a notion that with the increasing level of the compensation it is progressively more difficult to properly center the CSH containing a matching sample with respect to the sensing coil (i.e. in the center of the sample centering window of the MPMS software). All inaccuracies in the sample mounting inside the gap of the CSH and the other possible inhomogeneities, both of the shape of the substrate and/or of the investigated magnetic component, are causing strong deviations from the expected $\Upsilon(z)$-like shape, as exemplified in panels (a-c) of Fig. S3 - rendering the proper centering of the sample in a standard way practically impossible. The best way to circumvent this serious obstacle is to execute the centering procedure for the empty CSH before mounting of the investigated sample. Then, no further adjustments are needed after reloading of the whole sample holder assembly with the sample into the magnetometer. Of course, it is advisable to run the centering scan to confirm that the specimen remains in place. However, as long as the sample transport mechanism works according to the specifications, no additional position adjustment should be made, even if the displayed $V(z)$ in the MultiVu's centering window assumes a fairly bizarre shape - suggestive of a relocation of the sample to a different position. Such a conclusion might be inferred particularly from the example given in Fig. S3 (a), yet post-measurements centering test of the empty CSH reconfirmed the same position of the gap, and so the proper sample location with respect to the pick-up coils. Another confirmation of the proper centering can be occasionally obtained while running the measuring sequence when the total flux from the substrate and the gap becomes much smaller than that of the researched magnetic system (if such is investigated). This frequently happens at weak magnetic fields when the magnetic layer exhibits a sizable nonlinear behavior, characteristic for strongly interacting systems.

The inevitable distortion of measured $V(z)$, particularly for strong compensations, is the main reason that for the whole suite of the required measurements the magnetic moment should be established in the "linear" mode, that is when the least-squares regression of the model $\Upsilon(z)$ into the $V(z)$ is performed under internally set constrains that the magnetic flux originates from the central position in the pickup-coils. It needs to be underline here that although the MPMS system provides three procedures for data reduction: a *full scan* algorithm, a *maximum slope method*, and a *least-squares regression* (see ref. 5 and the discussion in ref. 3), without any doubts, only the last one is suitable for reliable minute moments magnetometry.[4]

The issue of adequate centering of the CSH and the necessity of limiting of the data reduction exclusively to the "linear" mode of the least-squares regression resembles the situation commonly met during hard-axis $m(T,H)$ measurements of an anisotropic material below its anisotropy field, that is when an odd in $z$ component

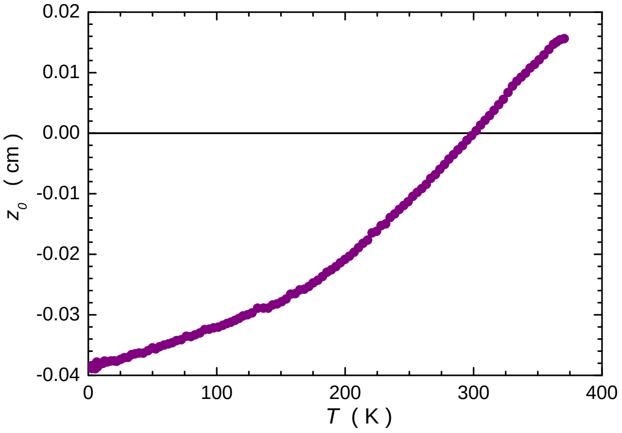


FIG. S5. A representative temperature dependence of the sample/gap position $z_0$ in a compensational sample holder established upon the measurement of the temperature dependence of the signal exerted by the empty gap between the compensating sapphire strips. This dependency has been established using the "iterative" mode for the data reduction, that is the least-squares regression was freed to search for the position of the maximum in $V(z)$.

considerably distorts $V(z)$ (c.f. Fig. 4 and the discussion in ref. 4). In both cases correct magnitudes of $m$ yielded in such an experimental frame is assured by the strictly even character of $\Upsilon(z)$. This seems to be a sufficiently unique feature differentiating the sought signal coming from the centrally located sample from all other "signals" contributing to the measured $V(z)$. In particular, the very well obeyed linear dependence of $\alpha_L$ on $\mu_{\mathrm{x}}\gamma_{\mathrm{x}}$ for the samples with $\mu_{\mathrm{x}}\gamma_{\mathrm{x}} \simeq \mu_{\mathrm{G}}\gamma_{\mathrm{G}}$, as presented in Fig. S3, strongly endorses this supposition.

Interestingly, the described above procedure works well in the whole temperature range of the magnetometer, despite the well-known fact that the sample changes its location with respect to the pick-up coils upon changes of $T$ due to the thermal contraction or expansion of the whole sample support. The effect is not by all means marginal, but is eliminated when the measurements are performed in the frame set by Eq. 2 (given and detailed in the main text). Concerning the absolute magnitude of this effect we note, as documented in Fig. S5, that for a CSH made of crystalline components (Si and/or sapphire) attached to the standard graphite sample rod, the sample position does not change with respect to 300 K, i.e. where the centering takes place, by more than 0.04 cm when $T$ is reduced to 2 K and the change is less than 0.02 cm during the $T$-trip to 400 K. The corresponding error of $m$ when working in the "linear" mode for a sample off-centered by 0.04 cm amounts to about 0.2%. Such a discrepancy is prohibitive for a precise magnetometry in general, but with the *in situ* substrate compensation this relative error bar applies only to the uncompensated part of the specimens' response - mainly to the magnetic layer in question, and so is perfectly acceptable. For these reasons there is no need to launch the MPMS sample "autotracking" option - designed to compensate for sample rod thermal expansion or contraction, in particular that this option is prone to induce some instabilities when measuring very low signals.[6] Secondly, the inaccuracies connected with working in the "linear" mode are either nearly identical for both the measurements of the sample and the reference and so they cancel out, or are strongly reduced by $\beta$ factor in Eq. 2. This is in fact another important advantage of the proposed here method of measurements. It indeed allows to work with the results provided directly by the MultiVu software. Contrary to the differential method[7], the sample position is evaluated beforehand and firmly set at the well-defined position ($z_0 = 2$ cm at $T = 300$ K) for all three required by Eq. 2 measurements, so there is no need to adjust $z_0$ numerically by an externally executed numerical routine.

According to the gained experience it is highly advisable to perform the pre-measurement centering routine always at the same $T$ and $H$. The authors choice has been 300 K and 20 kOe, respectively, the latter always ramped up from $H \simeq 0$.

* kgas@ifpan.edu.pl
† mikes@ifpan.edu.pl
1 A. Zieba, "Image and sample geometry effects in SQUID magnetometers," Rev. Sci. Instrum. **64**, 3357 (1993).
2 L. L. Miller, "The response of longitudinal and transverse pickup coils to a misaligned magnetic dipole," Rev. Sci. Instrum. **67**, 3201 (1996).
3 P. Stamenov and J. M. D. Coey, "Sample size, position, and structure effects on magnetization measurements using second-order gradiometer pickup coils," Review of Scientific Instruments **77**, 015106 (2006), https://doi.org/10.1063/1.2149190.
4 M. Sawicki, W. Stefanowicz, and A. Ney, "Sensitive SQUID magnetometry for studying nanomagnetism," Semicon. Sci. Technol. **26**, 064006 (2011).
5 Quantum Design, "The regression value algorithm," MPMS Application Note , 1014–214 (2001).
6 F. Bolzoni, S. Giraudo, L. Lopiano, B. Bergamasco, M. Fasano, and P.R. Crippa, "Magnetic investigations of human mesencephalic neuromelanin," Biochim. Biophys. Acta **1586**, 210 (2002).
7 R Cabassi, F Bolzoni, and F Casoli, "Differential method for sample holder background subtraction in superconducting quantum interference device (SQUID) magnetometry," Measurement Science and Technology **21**, 035701 (2010).
